# Supplementary material for: Lithography Hotspot Detection via Heterogeneous Federated Learning with Local Adaptation
Source: arXiv:2107.04367 source file (2021-07-30)
Supplement: Supplementary file 1 [file 8_appendix.tex]

\section{Appendix}
\subsection{Proof of Lemma~\ref{lem:bounded_consensus}}
% Before proceeding to prove the main theorem, we present two lemmas which are crucial to subsequent analysis. For brevity, we use the following auxiliary variables:
Let $(\hat{w}_{0,g}^{k},\hat{w}_{0,l}^{k} ) :=( w_{t,g}^{k},w_{t,l}^{k}),  k = 1,\cdots,N$ denote the variables at the beginning of each round of client's update and $\hat{\bar{w}}_{\cdot,g}=\frac{1}{N}\sum_{k=1}^N\hat{w}_{\cdot,g}^{k}$ denote the average.
% \begin{Lem}[Block-wise descent lemma~\cite{2013On}]\label{lem:block_descent}
% Suppose Assumptions 1-3 hold, then for all $w_l\in \mathbb{R}^{p_1}, w_g\in \mathbb{R}^{p_2}$, we have 
% \begin{equation*}
% \begin{aligned}
% &F_k\left( w_g, w_l+w \right) -F_k\left( w_g, w_l \right)  
% \\
% &~~~\leqslant \left< \nabla _l F_k\left( w_g, w_l \right) ,w \right> +\frac{L}{2}\left\| w \right\| ^2,
% % ~\forall w_l,w\in \mathbb{R}^{p_1}, w_g\in \mathbb{R}^{p_2},
% \end{aligned}
% \end{equation*}
% for local parameters, and 
% \begin{equation*}
% \begin{aligned}
% &F_k\left( w_g+w, w_l \right) -F_k\left( w_g, w_l \right)
% \\
% &~~~\leqslant \left< \nabla _g F_k\left( w_g, w_l \right) ,w \right> +\frac{L}{2}\left\| w \right\| ^2,
% % ~\forall w_l\in \mathbb{R}^{p_1}, w_g,w\in \mathbb{R}^{p_2},
% \end{aligned}
% \end{equation*}
% for global parameters.
% \end{Lem}
% \begin{IEEEproof}
Using the fact that $\mathbb{E}( \left\| X-\mathbb{E}X \right\| ^2 ) \leqslant \mathbb{E}( \left\| X \right\| ^2 ) $, we have \Cref{eq:app-1}.
\begin{figure}[htb!]
    \begin{equation}
        \begin{aligned}
        \label{eq:app-1}
            &\mathbb{E}\sum_{k=1}^N{\left\| \frac{1}{N}\sum_{j=1}^N{\hat{w}_{E,g}^{j}}-\hat{w}_{E,g}^{k} \right\| ^2} \\
            &\leqslant \mathbb{E}\sum_{k=1}^N{\left\| \hat{w}_{E,g}^{k}-\hat{\bar{w}}_{0,g}-\left( \hat{\bar{w}}_{E,g}-\hat{\bar{w}}_{0,g} \right) \right\| ^2} \\
            &\leqslant \mathbb{E}\sum_{k=1}^N{\left\| \hat{w}_{E,g}^{k}-\hat{\bar{w}}_{0,g} \right\| ^2} \\
            &\leqslant \mathbb{E}\sum_{k=1}^N{\left\| \eta \sum_{j=0}^{E-1}{\nabla _gF_k\left( \hat{w}_{j,g}^{k},\hat{w}_{j,l}^{k};\xi _{j}^{k} \right)} \right\| ^2}
        \end{aligned}
    \end{equation}
\end{figure}
Further, by Assumption 3, we have
\begin{equation*}
\begin{aligned}
&\mathbb{E}\sum_{k=1}^N{\left\| \frac{1}{N}\sum_{j=1}^N{\hat{w}_{E,g}^{j}}-\hat{w}_{E,g}^{k} \right\| ^2}
\\
&\leqslant \mathbb{E}\sum_{k=1}^N{\eta ^2\left( E-1 \right) ^2G^2}=\eta ^2N\left( E-1 \right) ^2G^2
\end{aligned}
\end{equation*}
which completes the proof.
% \end{IEEEproof}

% Lemma 3 is commented
\begin{comment}
\begin{Lem}[\textcolor{red}{can be absorbed in to the main proof}]
Suppose Assumption 1-3 hold, then for $\forall j\in \left[ 1,E \right]$, we have
\begin{equation*}
\begin{aligned}
&\sum_{k=1}^N{\mathbb{E}\left[ \left\| \nabla _lF_k\left( \hat{w}_{j-1,g}^{k},\hat{w}_{j-1,l}^{k} \right) \right\| ^2+\left\| \nabla _gF_k\left( \hat{w}_{j-1,g}^{k},\hat{w}_{j,l}^{k} \right) \right\| ^2 \right]}
\\
&\geqslant \frac{1}{2}\sum_{k=1}^N{\mathbb{E}\left[ \left\| \nabla F_k\left( \hat{w}_{j-1,g}^{k},\hat{w}_{j-1,l}^{k} \right) \right\| ^2 \right]}-N\eta ^2L^2G^2
\end{aligned}
\end{equation*}
\end{Lem}

\begin{IEEEproof}
According to Assumption 1, 3 and Lemma 2, for $j \in[1,E]$, we have
\begin{equation*}
\begin{aligned}
&\left\| \nabla _gF_k\left( \hat{w}_{j-1,g}^{k},\hat{w}_{j-1,l}^{k} \right) \right\| ^2
\\
&\leqslant 2\eta ^2L^2G^{2} +2\left\| \nabla _gF_k\left( \hat{w}_{j-1,g}^{k},\hat{w}_{j,l}^{k} \right) \right\| ^2
\end{aligned}
\end{equation*}
The rest of the proof is straightforward.
\end{IEEEproof}
\end{comment}

\subsection{Proof of Theorem 1}\label{Appdix}
Using Block-wise descent lemma~\cite{2013On}, we have, for $j=1,\cdots,E$,
\begin{equation*}
\begin{aligned}
&\mathbb{E}\left[ \sum_{k=1}^N{F_k\left( \hat{w}_{j-1,g}^{k},\hat{w}_{j,l}^{k} \right)}-\sum_{k=1}^N{F_k\left( \hat{w}_{j-1,g}^{k},\hat{w}_{j-1,l}^{k} \right)} \right] 
\\
&\leqslant \frac{\eta ^2LN}{2}G^{2}-\eta \sum_{k=1}^N{\mathbb{E}\left[ \left\| \nabla _l F_k\left( \hat{w}_{j-1,g}^{k},\hat{w}_{j-1,l}^{k} \right) \right\| ^2 \right]}
\end{aligned}
\end{equation*}
for local updates, and 
\begin{equation*}
\begin{aligned}
&\mathbb{E}\left[ \sum_{k=1}^N{F_k\left( \hat{w}_{j,g}^{k},w_{j,l}^{k} \right)}-\sum_{k=1}^N{F_k\left( \hat{w}_{j-1,g}^{k},w_{j,l}^{k} \right)} \right] 
\\
&\leqslant \frac{\eta ^2LN}{2}G^2-\eta \sum_{k=1}^N{\mathbb{E}\left[ \left\| \nabla _gF_k\left( \hat{w}_{j-1,g}^{k},\hat{w}_{j,l}^{k} \right) \right\| ^2 \right]}
\end{aligned}
\end{equation*}
for global updates.

Then, for $j=E+1$, we further have
\begin{equation*}
\begin{aligned}
&\mathbb{E}\left[ \sum_{k=1}^N{F_k\left( \hat{w}_{E,g}^{k},\hat{w}_{E+1,l}^{k} \right)}-\sum_{k=1}^N{F_k\left( \hat{w}_{E,g}^{k},\hat{w}_{E,l}^{k} \right)} \right] 
\\
&\leqslant \frac{\eta ^2LN}{2}G^2-\eta \sum_{k=1}^N{\mathbb{E}\left[ \left\| \nabla _lF_k\left( \hat{w}_{E,g}^{k},\hat{w}_{E,l}^{k} \right) \right\| ^2 \right]}
\end{aligned}
\end{equation*}
for local updates, and, with Lemma~\ref{lem:bounded_consensus},  
\begin{equation*}
\begin{aligned}
&\mathbb{E}\left[ \sum_{k=1}^N{F_k\left( \hat{w}_{E+1,g},\hat{w}_{E+1,l}^{k} \right)}-\sum_{k=1}^N{F_k\left( \hat{w}_{E,g}^{k},\hat{w}_{E+1,l}^{k} \right)} \right] 
\\
&\leqslant \eta \sqrt{N}\left( E-1 \right) G\sum_{k=1}^N{\left( \begin{array}{c}
	\left\| \nabla F_k\left( \hat{w}_{E,g}^{k},\hat{w}_{E+1,l}^{k} \right) \right\|\\
\end{array} \right)}
\\
&+\eta ^2LN\left( E-1 \right) ^2G^2+\eta ^2LNG^2
\\
&-\frac{\eta}{N}\left\| \sum_{k=1}^N{\nabla _gF_k\left( \hat{w}_{E,g}^{k},\hat{w}_{E+1,l}^{k} \right)} \right\| ^2.
\end{aligned}
\end{equation*}

Summing up all the above $2(E+1)$ inequalities we have
\begin{equation}\label{Eq_8}
\begin{aligned}
&\mathbb{E}\left[ \sum_{k=1}^N{F_k\left( \hat{w}_{E+1,g},\hat{w}_{E+1,l}^{k} \right)}-\sum_{k=1}^N{F_k\left( \hat{w}_{0,g}^{k},\hat{w}_{0,l}^{k} \right)} \right] 
\\
&\leqslant \eta \sqrt{N}\left( E-1 \right) G\sum_{k=1}^N{\left( \begin{array}{c}
	\left\| \nabla F_k\left( \hat{w}_{E,g}^{k},\hat{w}_{E+1,l}^{k} \right) \right\|\\
\end{array} \right)}
\\
&-\eta \sum_{j=1}^E{\sum_{k=1}^N{\mathbb{E}\left[ \begin{array}{c}
	\left\| \nabla _lF_k\left( \hat{w}_{j-1,g}^{k},\hat{w}_{j-1,l}^{k} \right) \right\| ^2\\
\end{array} \right]}}
\\
&-\eta \sum_{j=1}^E{\sum_{k=1}^N{\mathbb{E}\left[ \begin{array}{c}
	\left\| \nabla _gF_k\left( \hat{w}_{j-1,g}^{k},\hat{w}_{j,l}^{k} \right) \right\| ^2\\
\end{array} \right]}}+\mathcal{O}\left( \eta LG^2 \right).
\end{aligned}
\end{equation}
Noticing that 
\begin{equation*}
\begin{aligned}
&\left\| \nabla _gF_k\left( \hat{w}_{j-1,g}^{k},\hat{w}_{j-1,l}^{k} \right) \right\| ^2
\\
&\leqslant 2\eta ^2L^2G^{2} +2\left\| \nabla _gF_k\left( \hat{w}_{j-1,g}^{k},\hat{w}_{j,l}^{k} \right) \right\| ^2
\end{aligned}
\end{equation*}
and summing up (\ref{Eq_8}) from $t=0$ to $T-1$ and letting $w_{t+1}^{k} =[\hat{w}_{E+1,g}^{k}, \hat{w}_{E+1,l}^{k}]$,
then we have
\begin{equation*}
\begin{aligned}
&\frac{1}{T}\sum_{t=0}^{T-1}{\frac{1}{N}\sum_{k=1}^N{\left[ \left\| \nabla F_k\left( w_{t}^{k} \right) \right\| ^2 \right]}}
\\
&~~~\leqslant \frac{2\left[ \frac{1}{N}\sum_{k=1}^N{F_k\left( w_{0}^{k} \right)}-F^* \right]}{T\eta}
\\
&~~~+\mathcal{O}\left( \eta LG^2 \right) +2\sqrt{N}\left( E-1 \right) G\left( \sigma ^2+G^2 \right). 
\end{aligned}\textbf{}
\end{equation*}
